# Supplementary material for: Entanglement, Soft Modes, and Celestial CFT
Source: arXiv:2403.13913 source file (2024-03-20)
Supplement: Supplementary file 1 [file appendixB_innerProducts.tex]

\section{Inner products}
\label{app:ip}

This appendix should serve as a comprehensive guide to the inner product
computations needed. We define the Klein-Gordon product of two complex
scalar fields as
\begin{equation}
  \langle \Phi_1, \Phi_2\rangle = -i \int d^3 X \left[\Phi_1\partial_{X^0}\Phi_2^* - \partial_{X^0}\Phi_1 \Phi_2^* \right]. 
\end{equation}
The normalization is such that plane waves obey
\begin{equation}
  \begin{split}
    \langle e^{\pm iq \cdot X}, e^{\pm i q'\cdot X} \rangle &= - i \int d^3 X \left[\pm i q^{0'} e^{\pm i (q - q')\cdot X} \pm i q^0 e^{\pm i (q - q')\cdot X} \right]\\
                                                            &= \pm 2 (2\pi)^3 q^0 \delta^{(3)}(\vec{q} - \vec{q}').
  \end{split}
\end{equation}
This ensures that modes of a free scalar field $\Phi$ obey the canonical
commutation relations
\begin{equation}
  [a_{\vec{q}}, a^{\dagger}_{\vec{q}'}] =  2(2\pi)^3q^0 \delta^{(3)}(\vec{q} - \vec{q}').
\end{equation}
To see this, note that imposing the equal time commutation relations of the
field $\Phi$,
\begin{equation}
  [\Phi(X), \dot{\Phi}^*(X')] = \delta^{(3)}(X - X')
\end{equation}
{\color{red} [recheck this ]} leads to
\begin{equation}
  [a_{\vec{q}},  a^{\dagger}_{\vec{q}'}] = [\langle \Phi, e^{+iq\cdot X} \rangle, \langle e^{iq' \cdot X},  \Phi \rangle] = \langle e^{iq\cdot X}, e^{iq' \cdot X} \rangle = 2(2\pi)^3 q^0\delta^{(3)}(\vec{q} - \vec{q}').
\end{equation}
In the parameterization of the null momenta
\begin{equation}
  q(\omega, z, \bz) = \omega \nullUnit(z, \bz)
\end{equation}
we find that
\begin{equation}
  q^0\delta^{(3)}(\vec{q} - \vec{q}') = \omega^{-1} \delta(\omega - \omega') \delta^{(2)}(z - z').
\end{equation}

The generalization to spinning fields follows from {\color{red} [fill in
  details].}

For gauge fields, we hence have
\begin{equation}
\label{eq:scri-ip}
\langle A, A'\rangle = -i \int d\Sigma^{\mu}\left[A^{\nu} F^{'*}_{\mu\nu} -
  A^{'*\nu} F_{\mu\nu} \right].
\end{equation}

\subsection{Soft inner products at $\mathcal{I}^+$}

In this appendix we compute the inner products of bulk gauge fields with
Goldstone and Conformally Soft wavefunctions starting from the inner product
with a conformal primary wavefunction of generic $\confDim$ and taking the
corresponding limits \labelcref{eq:G-wf,eq:CS}. We will be exclusively
working with the parameterization of momenta in \cref{eq:null-vector}.

We start with the plane wave expansion
\begin{equation}
  A_{\mu}(X) = e \sum_{\alpha = \pm} \int \frac{d^3q}{(2\pi)^3 2\omega} \left( \polar_{\mu}^{*\alpha} a_{\alpha} e^{i\omega q\cdot X} + \polar_{\mu}^{\alpha} a^{\dagger}_{\alpha}e^{-i\omega q\cdot X} \right)
\end{equation}
as well as the definition of conformal primary wavefunctions
\begin{equation}
  A^{\confDim}_{a; \mu}(q; X_{\pm}) = \frac{\confDim - 1}{\confDim} \frac{\polar_{a;\mu}}{(- q \cdot X_{\pm})^{\confDim}} + \partial_{\mu} \alpha_a^{\confDim, \pm}.
\end{equation}
We have shown previously that $\partial_{\mu} \alpha_{\confDim}$ has no overlap with
$A_{\mu}$ for generic $\confDim,$ so we can effectively write (for generic
$\confDim$)
\begin{equation}
  \label{eq:Mellin}
  A^{\confDim}_{a; \mu}(q; X_{\pm}) \sim \frac{(\pm i)^{\confDim} \polar_{a;\mu}}{\confDim \Gamma(\confDim - 1)} \int_0^{\infty} \diff\omega \omega^{\confDim - 1} e^{\pm i\omega q\cdot X_{\pm}}.
\end{equation}
It will be useful to recall that
\begin{equation}
  \polar_{a;\mu} \polar_{b}^{*\mu} = \delta_{ab}, \quad \polar_{a;\mu}^* = \polar_{\bar{a};\mu}. 
\end{equation}
Then we find that
\begin{equation}
  \label{eq:Vip}
  \langle A^{\confDim \pm}_{a;\mu}(q'; X), \polar_{b}^{\mu} e^{\pm i \omega \nullUnit \cdot X} \rangle =  \pm(\celMet)_{a\bar{b}} \frac{(\pm i)^{\confDim}}{\confDim \Gamma(\confDim - 1)}  \omega^{\confDim - 2} 2 (2\pi)^3  \delta^{(2)}(z - z').
\end{equation}
% More details on our conventions can be found in \cref{app:ip}.
from which we obtain
\begin{equation}
  \label{eq:cpw-ip-A}
  \begin{split}
    \langle A^{+ \confDim}_{a;\mu}(q), A^{\mu}\rangle
    &= \frac{i^{\confDim} }{\confDim \Gamma(\confDim - 1)}
      \int_0^{\infty} \diff\omega \omega^{\confDim - 1}  e
      \sum_{\alpha = \pm} \int \frac{d^3q'}{(2\pi)^3 2\omega'} \polar_{\mu, \alpha}^{*} \polar_{a;\mu} a^{\alpha} \langle e^{i\omega q\cdot X_{+}}, e^{i\omega' q'\cdot X}\rangle\\
    &= \frac{i^{\confDim} }{\confDim \Gamma(\confDim - 1)} \int_0^{\infty} \diff\omega \omega^{\confDim - 1}  e  \int \frac{d^3q'}{(2\pi)^3 2\omega'} a_{a} \langle e^{i\omega q\cdot X_{+}}, e^{i\omega' q'\cdot X}\rangle\\ 
    &= \frac{i^{\confDim} }{\confDim \Gamma(\confDim - 1)} e \int_0^{\infty} \diff\omega \omega^{\confDim - 1}  a_a(\omega \nullUnit)\Ana{e^{-\reg \omega}},\\
    \langle A^{- \confDim}_{a;\mu}(q), A^{\mu}\rangle &= \frac{(- i)^{\confDim} }{\confDim \Gamma(\confDim - 1)} \int_0^{\infty} \diff\omega \omega^{\confDim - 1}  e \int \frac{d^3q'}{(2\pi)^3 2\omega'}  a^{\dagger}_{\bar{a}} \langle e^{-i\omega q\cdot X_{-}}, e^{-i\omega' q'\cdot X}\rangle\\ 
    &= -\frac{(- i)^{\confDim} }{\confDim \Gamma(\confDim - 1)} e \int_0^{\infty} \diff\omega \omega^{\confDim - 1} a^{\dagger}_{\bar{a}}(\omega\nullUnit) \Ana{e^{-\reg \omega}}.
  \end{split}
\end{equation}

We define the Goldstone wavefunction as
\begin{equation}
  A^G_{a;\mu} = \lim_{\confDim \rightarrow 1}\frac{1}{2e}\left[  A^{+ \confDim}_{a;\mu}(\nullUnit) + A^{- \confDim}_{a;\mu}(\nullUnit)\right]
\end{equation}
and the conformally soft wavefunction as
\begin{align}
  \begin{split}
    A^{CS}_{a;\mu} &= \frac{1}{2\pi i} \lim_{\confDim \rightarrow 1} \partial_{\confDim}\left[ A^{+ \confDim}_{a;\mu}(\nullUnit) - A^{- \confDim}_{a;\mu}(\nullUnit) \right] + {\rm shadow}\\
                   &= \frac{1}{2\pi i} \lim_{\confDim \rightarrow 1} \int \frac{d^2w}{2\pi} \p^b\partial_a \log|z - w|^2 \partial_{\confDim}\left[ A^{+ \confDim}_{b;\mu}(\nullUnit) - A^{- \confDim}_{\bar{b};\mu}(\nullUnit) \right],
  \end{split}
  \label{eq:conformally-soft-wf}
\end{align}
where here and henceforth $\partial_a, \partial_b$ are derivatives with respect to $z$ or
$\bz$. This allows us to write the conformally soft operator
\begin{equation}
  \label{eq:net-charge}
  \hat{\mathscr{Q}}_a \equiv -i\langle A^G_{a;\mu}, A^{\mu} \rangle = \frac{1}{2} \lim_{\omega \rightarrow 0} \omega \left[a_a(\omega \nullUnit) + a_{\bar{a}}^{\dagger}(\omega \nullUnit) \right]
\end{equation}
\Ana{[Note that this formula does not depend on $\reg$]} and the Goldstone
operator
\begin{align}
  \begin{split}
    \hat{\mathscr{S}}_a \equiv -i \langle A^{CS}_{a;\mu}, A^{\mu} \rangle
    &=  \frac{e}{2\pi i}\int_0^{\infty} \diff\omega \int \frac{d^2w}{2\pi} \p^{b}\partial_a\log|z - w|^2 \left[a_{b}(\omega, w) - a^{\dagger}_{\bar{b}}(\omega, w) \right] \Ana{e^{-\reg \omega}} \\
    &+ \frac{e}{2\pi i} \int \frac{d^2 w}{2\pi} \p^{b}\partial_a\log|z - w|^2  \lim_{\omega \rightarrow 0} \omega \Big[ -\frac{\pi}{2}\left((a_b(\omega,w) + a^{\dagger}_{\bar{b}}(\omega, w)\right)\\
    &-i\left(a_b(\omega, w) - a_{\bar{b}}^{\dagger}(\omega,w) \right) + i\log \omega \left(a_b(\omega, w) - a^{\dagger}_{\bar{b}}(\omega, w) \right) \Big],
  \end{split}
  \label{eq:Golstone-mode}
\end{align}
where in the second line we have used that $i^{\confDim} = e^{\frac{i\pi
    \confDim}{2}},~(-i)^{\confDim} = e^{-\frac{i\pi \confDim}{2}}$. \added[id=hzc]{[The
$\int \frac{d^2w}{2\pi} \partial^b \partial_a \log|z-w|^2$ in the second line
can actually be dropped, using the fact that $A^G$ and hence the soft charge are
total derivatives in the spherical directions.]}

Note that the first line in \cref{eq:Golstone-mode} agrees (up to
normalization) with the Goldstone operator derived in
\cite{Arkani-Hamed:2020gyp}. The other lines are proportional to zero-frequency
modes and their presence is sensitive to the order of limits employed in the
calculation of the inner product of the bulk gauge field with the conformally
soft modes. In particular, they are absent if one \deleted[id=hzc]{directly}
evaluates the inner product \added[id=hzc]{of individual plane waves} with
\cref{eq:conformally-soft-wf} \added[id=hzc]{then, after multiplying by
  creation and annihilation operators, integrates over all plane wave modes}.
This is the prescription adopted in the literature \cite{Arkani-Hamed:2020gyp}
which we review in the derivation of \cref{eq:GCS-ip} below.
\added[id=hzc]{However, this prescription is not sensitive to shifts of the
  Goldstone wavefunction by pure gauge $A^{CS}_{a;\mu} \to A^{CS}_{a;\mu} +
  \partial_{\mu} (\celMet)_{a}$, because the inner product between any pure gauge
  $\partial_\mu(\celMet)_a$, asymptotic or not, and any single plane wave vanishes.
  In fact, we shall argue that the first line on the RHS of \cref{eq:Golstone-mode}
  corresponds to $-i\langle A^{CS}_a - \frac{e}{2} A^G_a, A \rangle$.}
\replaced[id=hzc]{In contrast, we see in \cref{eq:Golstone-mode}}{Here we see}
that if we instead first evaluate the inner product of the gauge field with the
conformal primary wavefunctions using \cref{eq:cpw-ip-A} and finally take
$\partial_{\confDim}$ and $\confDim \rightarrow 1$, we obtain \deleted[id=hzc]{two}
additional contributions: a term proportional to \deleted[id=hzc]{a linear combination of} the
soft charge \labelcref{eq:net-charge} \deleted[id=hzc]{and its shadow}, and
\replaced[id=hzc]{terms proportional to the zero-frequency limit of
  $a(\omega)-a^\dagger(\omega)$}{the zero-frequency component of the
  conventional Goldstone operator (ie. the first line of
  \labelcref{eq:Golstone-mode})}. The former contribution \replaced[id=hzc]{is
  precisely $\frac{i e}{2}\langle A^G_a,A \rangle$.}{can be traced back to an
  ambiguity in the definition of the conformally soft wavefunction whose inner
  product with the Goldstone wavefunction determines it \textit{up~to} a pure
  gauge piece, $ A^{CS}_{a;\mu} \sim A^{CS}_{a;\mu} + \partial_{\mu} \beta_{a}$. } As
for the latter contribution, ...??? \added[id=amr]{[Is it this last line that
  one obtains by considering earlier definitions of the Goldstone operator
  involving sums of the boundary values of gauge fields at $\mathscr{I}$
  \cite{}?]} \added[id=hzc]{[I suspect one of the reasons they are showing up is that we have been
  (carelessly?) dropping trivial gauge contributions. E.g.~the last line of
  \cref{eq:conformally-soft-wf} is only correct up to a trivial gauge term.
  Note that $\lim_{\omega\to 0} \omega (a - a^\dagger) \sim \langle
  A^{1,+}-A^{1,-},A \rangle$ but $A^{1,+}-A^{1,-}$ is trivial gauge
  (as it vanishes at the spacetime boundary).]}

% But now notice that the terms involving soft photons vanish. This follows from
% the identity \be \lim_{\omega \rightarrow 0} \omega \left( a_{\pm}(\omega,z) -
%   \int \frac{d^2w}{2\pi} \frac{1}{(z - w)^2} a_{\mp}(\omega, w)\right)
% {\color{red}\neq} 0. \end{equation} \Ana{[Need a $+$ in the final equality
% otherwise it doesn't work. There is something weird going on with the
% regulator for the shadow terms. If one analyzes the wavefunctions, there is a
% cancellation which doesn't seem to appear in A.16]}
% \begin{equation}
%   \int_0^{\infty} \diff\omega \left[a_a(\omega\nullUnit) -
%     a^{\dagger}_{\bar{a}}(\omega \nullUnit) \right] \end{equation} has no poles
% at $\confDim = 1$. To see this we note that
% \begin{equation}
%   \lim_{\confDim \rightarrow 1}(\confDim - 1) \int_0^{\infty}\diff\omega \langle
%   \hat{\mathscr{S}}_a \mathcal{O}_1 \cdots \rangle = \lim_{\omega \rightarrow
%   0} \omega \langle {\rm out}| a_a(\omega) S + S a^{\dagger}_{\bar{a}}(\omega)
%   |{\rm in}\rangle = 0 \end{equation} by crossing symmetry.

% II. We now derive the same results by computing the inner products of the
% conformal primary wavefunctions \eqref{} at $\mathcal{I}^+$ directly.

Assuming that the Goldstone operator is simply given by the first line in
\cref{eq:Golstone-mode}, we find that
\begin{equation}
  [\hat{\mathscr{S}}_a(z), \hat{\mathscr{Q}}_{\bar{b}}(z')] =- [\langle A^G_{a;\mu}, A^{\mu}\rangle, \langle A^{\mu}, A^{CS}_{\bar{b};\mu} \rangle] = -e^2\langle A^G_a, A^{CS}_{\bar{b}}\rangle =  -4\pi i e \partial_a \partial_{\bar{b}} \log|z - z'|^2.
\end{equation}
{\color{red}[double check signs.]}
% {\color{red} [this seems to differ by a factor of $2\pi$ (probably made a
% mistake I can't find) as well as a shadow from other definitions... The shadow
% missing I am not too worried about, it was also already pointed out in
% \cite{}.]}
Had we instead expanded the conformal primary wavefunctions at large $r$ and
taken $\confDim = 1$ before evaluating the inner products, we would find
\begin{equation}
  A^G_{a;\mu} = \frac{1}{e}\partial_{\mu} \alpha_a , \quad  \alpha_a = \frac{\polar_a \cdot X_{\pm}}{(-\nullUnit \cdot X_{\pm})}
\end{equation}
% {\color{red} [I am confused again why we are allowed to drop the plane wave
% contribution, even using this prescription that seems to survive, gives a term
% $\propto \delta(\milneFreq)$.]}

At large $r$ the plane wave expansions take the form
\begin{equation}
  A^{\pm,P}_{\mu; a} = \polar_{\mu;a} e^{\pm i \omega( \nullUnit \cdot X \mp i\reg)} = \polar_{\mu}^{+} e^{\mp i \omega( u + r |z - w|^2 \mp i\reg)} \sim \mp i (\omega r)^{-1} \polar_{\mu}^{+} e^{\mp i \omega (u \mp i \reg)} (2\pi)^2\delta^{(2)}(z - w)
\end{equation}
and the expansion of the Goldstone wavefunction at large $r$
\begin{align}
  \begin{split}
    \partial_{\mu}\alpha_z &=  -\partial_{\mu}\frac{r (\bz - \bw)}{r|z - w|^2 + u} \\
    % &= \left( \frac{ r(\bz- \bw)}{(u + r|z - w|^2)^{2}}, \frac{(\bw - \bz) u}{(u + r|z - w|^2)^{2}}, -\frac{r^2(\bw - \bz)^2}{(u + r|z - w|^2)^{2}} , \frac{r u }{(u + r|z - w|^2)^{2}}\right)\\
& \rightarrow \left(\mathcal{O}(r^{-1}), \mathcal{O}(r^{-2}), -\frac{1}{(z - w)^2} + \mathcal{O}(r^{-1}), 2\pi \delta^{(2)}(z - w) + \mathcal{O}(r^{-1})\right).
\end{split}
  % \label{eq:palpha}
\end{align}
Evaluating the inner product of $A^G$ and $A^{CS} = e \Theta(-u) A^G$ directly at $\mathcal{I}^+$ we find using \cref{eq:scri-ip} 
%{\color{red} [I need to cross-check this]}
\begin{equation} 
\label{eq:GCS-ip}
\langle A^G_a, A^{CS}_{\bar{b}}\rangle =  \frac{4\pi i}{e} \partial_a \partial_{b} \log|z - z'|^2. 
\end{equation}

It will be useful to write down expressions for $\hat{\mathscr{Q}}_a$ and $\hat{\mathscr{S}}_a$ in terms of the conformal primary modes. To this end, we first work out the relation between plane wave and conformal primary modes 
\begin{equation} 
\begin{split}
a_{\bar{b}}(\omega \nullUnit) &= \frac{1}{e}\langle A_{\mu}, \polar_{b}^{\mu} e^{i\omega \nullUnit\cdot X} \rangle = \int_{-\infty}^{\infty} d\milneFreq \int d^2z'  \mu^{+}(\milneFreq) \langle A^{1 + i\milneFreq, +}_{\mu;a}, \varepsilon^{\mu}_b e^{i\omega \nullUnit\cdot X}\rangle a^a_{\milneFreq}(\nullUnit'), \\
a^{\dagger}_b(\omega \nullUnit) &= -\frac{1}{e}\langle A_{\mu}, \polar_{b}^{\mu} e^{-i\omega \nullUnit\cdot X} \rangle = -\int_{-\infty}^{\infty} d\milneFreq \int d^2z' \mu^{-*}(\milneFreq) \langle A^{1 - i\milneFreq, -}_{\mu;\bar{a}}, \varepsilon^{\mu}_b e^{-i\omega \nullUnit\cdot X}\rangle a^{a\dagger}_{\milneFreq}(\nullUnit').
\end{split}
\end{equation}
Using the inner product \labelcref{eq:Vip}, together with \cref{eq:norm}, we find
\begin{equation} 
\label{eq:pw-cpw}
\begin{split}
    a_{\bar{b}}(\omega \nullUnit) &= \int_{-\infty}^{\infty} d\milneFreq \mu^{+}(\milneFreq) \frac{i^{1 + i\milneFreq}}{(1 + i\milneFreq) \Gamma(i\milneFreq)} \omega^{i\milneFreq - 1} 2(2\pi)^3 e^{-\reg \omega} a_{\bar{b};\milneFreq}(\nullUnit)\\
    a^{\dagger}_b(\omega \nullUnit) &= \int_{-\infty}^{\infty} d\milneFreq \mu^{-*}(\milneFreq) \frac{(-i)^{1 - i\milneFreq}}{(1 - i\milneFreq) \Gamma(-i\milneFreq)} \omega^{-i\milneFreq - 1} 2(2\pi)^3 e^{-\reg \omega} a^{\dagger}_{b;\milneFreq}(\nullUnit).\\
\end{split}
\end{equation}
Finally, using the identity \cite{}
\begin{equation} 
\lim_{\omega \rightarrow 0} \omega^{\confDim - 1} = -2\pi (\confDim - 1) \delta(\confDim - 1)
\end{equation}
valid for $\confDim = 1 + i\milneFreq$ we find
\begin{equation} 
\begin{split}
    \hat{\mathscr{Q}}_b(z) &= \frac{2\sqrt{2}\pi^2 i}{e}\lim_{\milneFreq \rightarrow 0}\milneFreq\left( a_{b;\milneFreq}(z) - a_{\bar{b};-\milneFreq}^{\dagger}(z) \right), \\
    \hat{\mathscr{S}}_b &= \frac{i}{\sqrt{2}} \int \frac{d^2w}{2\pi} \p^{b}\partial_a\log|z - w|^2  \Ana{\int d\milneFreq \int_0^{\infty} \diff\omega\left[a_{b; \milneFreq}(w)+ a^{\dagger}_{\bar{b};-\milneFreq}(w) \right] \omega^{i\milneFreq-1}\left(\cdots \right) e^{-2\omega \reg}} .
\end{split}
\end{equation}
{\color{red} This is off by a factor of $\pi$ when $\reg \rightarrow 0$. I don't see why we cannot take $\reg \rightarrow 0$ here (and consistently so far), so the factor in red becomes $\delta(\milneFreq)$. }

\subsection{Left/right Milne patches}
\label{app:left-right-Milne}

We adopt the same approach before. We first compute the inner products of
of the bulk gauge fields $A$ with the left and right conformal primary
wavefunctions. To this end it will be useful to compute the KG product of
plane waves
\begin{equation} 
\begin{split}
\langle e^{\pm i \omega q\cdot X_{\pm}}, e^{\pm i\omega' q' \cdot X_{\pm}} \rangle_{L} &= (2\pi)^2i \int_0^{\infty} du  \left[\pm i\omega^{-1}e^{\mp i \omega(u \mp i \reg) \pm i\omega'(u \pm i\reg)} (\sqrt{{\rm det}\celMet})^{-1} \delta^2(z - z') +(\omega \leftrightarrow \omega')\right]\\
&= \mp(2\pi)^2 (\sqrt{{\rm det}\celMet})^{-1}  \delta(z - z') \omega^{-1}\frac{-i e^{-(\omega + \omega')\reg}}{\pm (\omega - \omega')-i\reg} + (\omega \leftrightarrow \omega')\\
\langle e^{\pm i \omega q\cdot X_{\pm}}, e^{\mp i\omega' q' \cdot X_{\mp}} \rangle_{L} &= \mp(2\pi)^2 (\sqrt{{\rm det}\celMet})^{-1} \delta(z - z') \omega^{-1}\frac{-ie^{-(\omega + \omega')\reg}}{\pm (\omega + \omega')-i\reg} + (\omega \leftrightarrow \omega'),\\
\langle e^{\pm i \omega q\cdot X_{\pm}}, e^{\pm i\omega' q' \cdot X_{\pm}} \rangle_{R} &= \mp(2\pi)^2 (\sqrt{{\rm det}\celMet})^{-1}  \delta(z - z') \omega^{-1}\frac{-i e^{-(\omega + \omega')\reg}}{\mp (\omega - \omega')-i\reg} + (\omega \leftrightarrow \omega'),\\
\langle e^{\pm i \omega q\cdot X_{\pm}}, e^{\mp i\omega' q' \cdot X_{\mp}} \rangle_{R} &= \mp(2\pi)^2 (\sqrt{{\rm det}\celMet})^{-1}  \delta(z - z') \omega^{-1}\frac{-ie^{-(\omega + \omega')\reg}}{\mp (\omega + \omega')-i\reg} + (\omega \leftrightarrow \omega'),
\end{split}
\end{equation}
where we used
\begin{equation}
 e^{\pm i \omega( \nullUnit \cdot X \mp i\reg)} = e^{\mp i \omega( u + r |z - w|^2 \mp i\reg)} = \mp i (\omega r)^{-1} e^{\mp i \omega (u \mp i \reg)} (2\pi)^2 (\sqrt{{\rm det}\celMet})^{-1}  \delta^{(2)}(z -w) 
\end{equation}
{\color{red} [CHECK overall sign]}

As a cross check we note that the sum of the left and right patch plane wave inner products gives the expected result
\begin{equation} 
\langle e^{\pm i \omega q\cdot X_{\pm}}, e^{\pm i\omega' q' \cdot X_{\pm}} \rangle = \pm (2\pi)^3 2 (\sqrt{{\rm det}\celMet})^{-1}  \omega^{-1}\delta(\omega - \omega') \delta(z - z'),
\end{equation}
with the other combinations vanishing since $\omega, \omega' > 0.$
We find that 
\begin{equation} 
\begin{split}
\langle A^{+L \confDim}_{a;\mu}(q), A_{\mu}\rangle 
&= \frac{i^{\confDim} e}{\confDim \Gamma(\confDim - 1)} \int_0^{\infty} \diff\omega \omega^{\confDim - 1} \\
&\times  \int \frac{d^3q'}{(2\pi)^3 2\omega'} \left[a_{a} \langle e^{i\omega q\cdot X_{+}}, e^{i\omega' q'\cdot X_{+}}\rangle_L + a_{\bar{a}}^{\dagger} \langle e^{i\omega q\cdot X_{+}}, e^{-i\omega' q'\cdot X_{+}}\rangle_L\right]\\ 
&= -\frac{i^{\confDim} e}{\confDim \Gamma(\confDim - 1)} \int_0^{\infty} \diff\omega \int_0^{\infty} \diff\omega' \omega^{\confDim - 1}  \frac{-i}{4\pi}\Big[\frac{\omega'}{\omega(\omega - \omega' - i\reg)}a_a(\omega' \nullUnit) \\
&+ \frac{\omega'}{\omega(\omega + \omega' - i\reg)}a_{\bar{a}}^{\dagger}(\omega' \nullUnit) + \frac{1}{(\omega' - \omega - i\reg)}a_a(\omega' \nullUnit) + \frac{1}{(\omega + \omega' - i\reg)}a_{\bar{a}}^{\dagger}(\omega' \nullUnit)\Big],\\
\langle A^{- L \confDim}_{a;\mu}(q), A_{\mu}\rangle &= \frac{(- i)^{\confDim} }{\confDim \Gamma(\confDim - 1)} e \int_0^{\infty} \diff\omega \int_0^{\infty} \diff\omega' \omega^{\confDim - 1}  \frac{-i}{4\pi}\Big[\frac{\omega'}{\omega(-\omega' - \omega - i\reg)}a_a(\omega' \nullUnit) \\
&+ \frac{\omega'}{\omega(-\omega + \omega' - i\reg)}a_{\bar{a}}^{\dagger}(\omega' \nullUnit) + \frac{1}{(-\omega' - \omega - i\reg)}a_a(\omega' \nullUnit) + \frac{1}{(-\omega' + \omega - i\reg)}a_{\bar{a}}^{\dagger}(\omega' \nullUnit) \Big]
\end{split}
\end{equation}
and similarily
\begin{equation} 
\begin{split}
\langle A^{+R \confDim}_{a;\mu}(q), A_{\mu}\rangle  &= -\frac{i^{\confDim} }{\confDim \Gamma(\confDim - 1)} e \int_0^{\infty} \diff\omega \int_0^{\infty} \diff\omega' \omega^{\confDim - 1}  \frac{-i}{4\pi}\Big[\frac{\omega' - \omega}{\omega(\omega' - \omega - i\reg)}a_a(\omega' \nullUnit) \\
&+ \frac{\omega' + \omega}{\omega(-\omega - \omega' - i\reg)}a_{\bar{a}}^{\dagger}(\omega' \nullUnit)\Big]
\\
\langle A^{- R \confDim}_{a;\mu}(q), A_{\mu}\rangle &= \frac{(- i)^{\confDim} }{\confDim \Gamma(\confDim - 1)} e \int_0^{\infty} \diff\omega \int_0^{\infty} \diff\omega' \omega^{\confDim - 1}  \frac{-i}{4\pi}\Big[\frac{\omega' + \omega}{\omega(\omega + \omega' - i\reg)}a_a(\omega' \nullUnit) \\
&+ \frac{\omega' - \omega}{\omega(\omega - \omega' - i\reg)}a_{\bar{a}}^{\dagger}(\omega' \nullUnit) \Big].
\end{split}
\end{equation}

We find the left and right Goldstone operators by taking the limits of the above as $\confDim \rightarrow 1.$ We get
\begin{equation}
\begin{split}
\langle A^{+L \confDim=1}_{a;\mu}(q), A_{\mu}\rangle 
&= \frac{e}{4\pi}\int_0^{\infty} \diff\omega \left[\frac{\omega}{\omega + i\reg}a_a(\omega \nullUnit) - \frac{\omega}{\omega - i\reg}a_{\bar{a}}^{\dagger}(\omega \nullUnit) \right]\\
 \langle A^{-L \confDim=1}_{a;\mu}(q), A_{\mu}\rangle &=  \frac{e}{4\pi}\int_0^{\infty} \diff\omega \left[\frac{\omega}{\omega + i\reg}a_a(\omega \nullUnit) - \frac{\omega}{\omega - i\reg}a_{\bar{a}}^{\dagger}(\omega \nullUnit) \right]\\
\langle A^{+R \confDim=1}_{a;\mu}(q), A_{\mu}\rangle 
&= -\frac{e}{4\pi}\int_0^{\infty} \diff\omega \left[\frac{\omega}{\omega - i\reg}a_a(\omega \nullUnit) - \frac{\omega}{\omega + i\reg}a_{\bar{a}}^{\dagger}(\omega \nullUnit)  \right] \\
\langle A^{-R \confDim=1}_{a;\mu}(q), A_{\mu}\rangle &= -\frac{e}{4\pi}\int_0^{\infty} \diff\omega \left[\frac{\omega}{\omega - i\reg}a_a(\omega \nullUnit) - \frac{\omega}{\omega + i\reg}a_{\bar{a}}^{\dagger}(\omega \nullUnit)  \right]. \\
\end{split}
\end{equation}
We see that adding up the left and right results we obtain \cref{eq:net-charge} as expected. We also see that in the limit $\reg \rightarrow 0$ these operators are proportional to the Goldstone operators (rather than the conformally soft ones).  

To compute the left and right Goldstone operators it will be convenient to first note that
\begin{equation} 
\begin{split}
\langle A^{+L \confDim}_{a;\mu}, A_{\mu}\rangle - \langle A^{-L \confDim}_{a;\mu}, A_{\mu}\rangle &= -\frac{i^{\confDim} }{\confDim \Gamma(\confDim - 1)} e \int_{-\infty}^{\infty} \diff\omega \int_0^{\infty} \diff\omega' \omega^{\confDim - 1}  \frac{-i}{4\pi}\Big[\frac{\omega' e^{-(\omega + \omega')\reg}}{\omega(-\omega' + \omega - i\reg)}a_a(\omega' \nullUnit) \\
&+ \frac{\omega' e^{-(\omega + \omega')\reg}}{\omega(\omega + \omega' - i\reg)}a_{\bar{a}}^{\dagger}(\omega' \nullUnit) + (\omega \leftrightarrow \omega')\Big]\\
\langle A^{+R \confDim}_{a;\mu}, A_{\mu}\rangle - \langle A^{-R \confDim}_{a;\mu}, A_{\mu}\rangle &= -\frac{i^{\confDim} }{\confDim \Gamma(\confDim - 1)} e \int_{-\infty}^{\infty} \diff\omega \int_0^{\infty} \diff\omega' \omega^{\confDim - 1}  \frac{-i}{4\pi}\Big[\frac{\omega' e^{-(\omega + \omega')\reg}}{\omega(\omega' - \omega - i\reg)}a_a(\omega' \nullUnit) \\
&+ \frac{\omega' e^{-(\omega + \omega')\reg}}{\omega(-\omega - \omega' - i\reg)}a_{\bar{a}}^{\dagger}(\omega' \nullUnit) + (\omega \leftrightarrow \omega')\Big].
\end{split}
\end{equation}

We now close the contour. We illustrate the calculation for one of the integrals and simply state the results for the rest
\begin{equation} 
\begin{split}
&-\frac{i^{\confDim} }{\confDim \Gamma(\confDim - 1)} e \int_{-\infty}^{\infty} \diff\omega \int_0^{\infty} \diff\omega' \omega^{i\milneFreq}  \frac{-i}{4\pi}\left[\frac{\omega' e^{-(\omega + \omega')\reg}}{\omega(-\omega' + \omega - i\reg)}a_a(\omega' \nullUnit) + (\omega \leftrightarrow \omega')\right]\\
&= -\frac{i^{\confDim} }{\confDim \Gamma(\confDim - 1)} e  \int_0^{\infty} \diff\omega' \omega'^{i\milneFreq}  \frac{-i}{4\pi}\left[a_a(\omega'\nullUnit)\Theta(\milneFreq) + a_a(\omega'\nullUnit)\Theta(-\milneFreq) \right]
\end{split}
\end{equation}
where for the first integral we close the contour in the UHP if $\milneFreq > 0$ and in the LHP for $\milneFreq <0$ hence the theta function. Similar for the second integral. 
{\color{red} Note that there is also a pole in $\omega$ (we have not dropped any $i\reg$ prescription). If we regulate $\confDim - 1 = \epsilon$ with $\epsilon > 0$ (as done for example in \cite{}), this contribution drops out. We will assume throughout that this prescription has been adopted. } Putting everything together we find
\begin{equation} 
\begin{split}
\langle A^{+L \confDim}_{a;\mu}(q), A_{\mu}\rangle - \langle A^{-L \confDim}_{a;\mu}(q), A_{\mu}\rangle &= -\frac{i^{\confDim}}{2\confDim \Gamma(\confDim - 1)} e \int_0^{\infty} \diff\omega \left[\omega^{i\milneFreq} a_a(\omega \nullUnit) - (-\omega)^{i\milneFreq}a_{\bar{a}}^{\dagger}(\omega\nullUnit) \right],\\
\langle A^{+R \confDim}_{a;\mu}(q), A_{\mu}\rangle - \langle A^{-R \confDim}_{a;\mu}(q), A_{\mu}\rangle &= -\frac{i^{\confDim}}{2\confDim \Gamma(\confDim - 1)} e \int_0^{\infty} \diff\omega \left[\omega^{i\milneFreq} a_a(\omega \nullUnit) - (-\omega)^{i\milneFreq}a_{\bar{a}}^{\dagger}(\omega\nullUnit) \right].
\end{split}
\end{equation}
As discussed before (assuming the linear combination of modes has no poles in $\confDim = 1$) we have
\begin{equation} 
\begin{split}
\lim_{\confDim \rightarrow 1} \partial_{\confDim}\left[\langle A^{+L \confDim}_{a;\mu}(q), A_{\mu}\rangle - \langle A^{-L \confDim}_{a;\mu}(q), A_{\mu}\rangle\right] &= - \frac{i e}{2}\int_0^{\infty} \diff\omega \left[ a_a(\omega \nullUnit) - a_{\bar{a}}^{\dagger}(\omega\nullUnit) \right],\\
\lim_{\confDim \rightarrow 1} \partial_{\confDim}\left[\langle A^{+R \confDim}_{a;\mu}(q), A_{\mu}\rangle - \langle A^{-R \confDim}_{a;\mu}(q), A_{\mu}\rangle \right] &= -  \frac{i e}{2}\int_0^{\infty} \diff\omega \left[a_a(\omega \nullUnit) - a_{\bar{a}}^{\dagger}(\omega\nullUnit) \right].
\end{split}
\end{equation}
{\color{red} [overall sign?]}
To see this in more detail, the left and right Goldstone operators are given by
\begin{equation} 
\begin{split}
\langle A^{CS, L}_{a;\mu}, A_{\mu} \rangle &= \frac{1}{2\pi i}\left[ \partial_{\confDim}\left[\langle A^{+L \confDim}_{a;\mu}(q), A_{\mu}\rangle - \langle A^{-L \confDim}_{a;\mu}(q), A_{\mu}\rangle\right] + {\rm shadow} \right]\\
& = \lim_{\confDim \rightarrow 1} \left[\partial_{\confDim} \frac{1}{\Gamma(\confDim - 1)} \left( \right) + \frac{1}{\Gamma(\confDim - 1)}\partial_{\confDim}\left( \right)\right]\\
\end{split}
\end{equation}
Where we expanded $(\pm i)^{\confDim}$ around $\confDim = 1$ and noted that the subleading terms have no poles at $\confDim = 1$ and hence vanish.

In terms of the conformal primary wavefunctions we find

%{\color{red} Derive the inner product by either taking $\omega \rightarrow 0$ first or $r \rightarrow \infty$ first.}

%%% Local Variables:
%%% mode: latex
%%% TeX-master: "../main"
%%% End:
