# Supplementary material for: Entanglement, Soft Modes, and Celestial CFT
Source: arXiv:2403.13913 source file (2024-03-20)
Supplement: Supplementary file 2 [file appendixC_coherentStates.tex]

\section{Coherent state identities}
\label{app:coh}

%%% Local Variables:
%%% mode: latex
%%% TeX-master: "../main"
%%% End:
