# Supplementary material for: Entanglement, Soft Modes, and Celestial CFT
Source: arXiv:2403.13913 source file (2024-03-20)
Supplement: Supplementary file 3 [file appendixD_oldSoftEntanglement.tex]

\section{Old stuff about entanglement of soft modes}
\label{sec:banana}

\subsection{Review of DW's edge modes}
Here, review the
calculation of the edge mode contribution to the vacuum entanglement entropy in
pure Maxwell theory \cite{Donnelly:2014fua, Donnelly:2015hxa}.

Consider the future Milne patch of Minkowski space depicted in \cref{fig:potato}.
This is covered by coordinates $(\tau, \rho, z_s, \bz_s)$ \cite{} in which the
Minkowski metric takes the form
\begin{equation}
  \label{eq:Milne-metric}
  ds^2 = e^{2\tau}\left(-d\tau^2 + d\rho^2 + \sinh^2 \rho d\Omega_2^2 \right),
\end{equation}
where $d\Omega_2^2$ is the metric on the unit 2-sphere. This metric is conformal
to $\mathbb{R} \times H^{3}$.

It will be convenient to trade the global $(\rho, z_z, \bz_s)$ coordinates on
$H_3$ for Poincar\'e coordinates $(\anas, w, \bw)$
\begin{equation}
  \begin{split}
    \cosh\rho = \left[\cosh \anas + e^{-\anas}w\bw \right], \quad z_s = \frac{2 \sqrt{2}w}{e^{2\anas} + 2w\bw + 2e^{\anas}\sinh \rho - 1 }
  \end{split}
\end{equation}
% {\color{red} recheck...}
in which case the metric on (half of) $H_3$ takes the form
\begin{equation}
  ds_{H_3}^2 = d\anas^2 + e^{-2\anas} 2dw d\bar{w}.
\end{equation}
Note that the relation between these Poincar\'e coordinates and the planar
retarded coordinates in \cref{eq:planar-Mink} is simply
\begin{equation}
  r = e^{-\sigma +
  \tau}, \quad u = e^{\tau + \sigma}, \quad z = w.
\end{equation}

% {\color{red} [See Poincare-new-2022 mathematica file]}

As illustrated in fig.~\ref{}, the entanglement entropy of edge modes across
the cut at $u = 0$ can be computed by evaluating the thermal entropy of the
Milne region \cite{}. By conformal symmetry the result
should be independent on $\tau$, hence we expect this to be the same as the
entanglement entropy across $\mathcal{I}^+$ corresponding to the limit $\tau
\rightarrow \infty$. We will confirm this by an explicit calculation at
$\mathcal{I}^+$ in section \ref{}. Following Donnelly and Wall (DW) \cite{}, the
edge mode entropy is extracted from the Euclidean partition
function
\begin{equation}
  \label{eq:edge-partition-fctn}
  Z_{\rm edge} = \int \mathcal{D} E_{\perp} e^{-I_{cl}(E_{\perp})},
\end{equation}
where $I_{cl.}$ is the on-shell action
\begin{equation}
  % \label{classical-action}
  I_{cl} = \frac{1}{2} \int_{\p M} A \wedge \star F
\end{equation}
and $E_{\perp}$ is the boundary value of the electric field which is kept fixed.
The boundary is taken to be the Euclidean circle at large $\rho = \rho_0$
(equivalently large negative $\sigma \rightarrow -\sigma_0$). For a static gauge
field in Lorenz gauge,
\begin{equation}
  \label{eq:ansatz}
  A = \sum_{\ell,m} \widetilde{R}_{\ell}(\sigma) Y_{\ell, m}(w, \bw) d\tau
\end{equation}
and
\begin{equation}
  \label{eq:eom}
  \Box A_{\tau} = 0 \iff \partial_{\sigma} \left(e^{-2\sigma} \partial_{\sigma} A_{\tau}
  \right) + 2 \partial_w\partial_{\bw} A_{\tau} = 0.
\end{equation}
Substituting \cref{eq:ansatz} into \cref{eq:eom}, we arrive at the following
differential equation for the radial wavefunction
$\widetilde{R}_{\ell}$
\begin{equation}
  \label{eq:radial-me}
  \partial_{\sigma} \left(e^{-2\sigma} \partial_{\sigma} \widetilde{R}_{\ell} \right) -
  \ell(\ell + 1) \widetilde{R}_{\ell} = 0,
\end{equation}
where we used the defining equation for the spherical harmonics
\begin{equation}
  2\partial_w\partial_{\bw} Y_{\ell, m}(w, \bw) = -\ell(\ell + 1) Y_{\ell, m}(w, \bw) .
\end{equation}

The solutions to \cref{eq:radial-me} are linear combinations of Bessel functions,
which to leading order at large $\rho$ expand as
\begin{equation}
  \label{eq:radial}
  \widetilde{R}_{\ell}(\sigma) = \widetilde{c}_2\left(1 + \frac{1}{2} \ell(\ell +
    1) e^{2\sigma} \sigma + \mathcal{O}(e^{2\sigma}) \right).
\end{equation}
Imposing that the electric field is constant at $\sigma = -\sigma_0$, and that
the net Milne charge \begin{equation}
 Q_M \equiv \int_{\sigma = \sigma_0} d^2w e^{2\sigma_0}
\widetilde{E}(w,\bw)
\end{equation}
is finite, we find
\begin{equation}
  % \label{e-field}
  \left. \widetilde{E} \right|_{\sigma = -\sigma_0}= \sum_{\ell,m} e^{-2\sigma_0}
  E_{\ell,m} Y_{\ell, m}(w,\bw),
\end{equation}
and hence at large positive $\sigma_0$
\begin{equation}
 \left. \int d^2w Y_{\ell, m}
  \widetilde{E} \right|_{\sigma = -\sigma_0} = E_{\ell, m} e^{-2\sigma_0}, \quad
\left. \partial_\sigma \widetilde{R}_{\ell} \right|_{\sigma = -\sigma_0} = E_{\ell, m}
e^{-2\sigma_0}= -\widetilde{c}_2 \ell(\ell + 1) e^{-2\sigma_0} \sigma_0.
\end{equation}
Then
\begin{equation}
 \widetilde{c}_2 = -\frac{E_{\ell, m}}{\ell(\ell + 1) \sigma_0}
\end{equation}
and therefore
\begin{equation}
  % \label{milne-euclidean-action}
  \widetilde{I}_{cl.} = \frac{1}{2} \int_{\sigma = -\sigma_0} \widetilde{A} \wedge
  \widetilde{\star} \widetilde{F} = -\frac{1}{2} \oint d\tau \int d^2w
  e^{2\sigma_0} \widetilde{A}_{\tau} \widetilde{F}_{\sigma\tau} = \sum_{\ell}
  \frac{\beta E_{\ell, m}^2}{2 \ell(\ell + 1) \sigma_0} .
\end{equation}

 
 
The remaining ingredient needed to evaluate the RHS of \cref{eq:edge-partition-fctn} is the
path integral measure. Upon discretization, this reduces to
\cite{}
\begin{equation} \mathcal{D} E_{\perp} = \prod_{\ell > 0, m} \frac{1}{q}
  \frac{1}{\sqrt{N}} dE_{\ell, m},
\end{equation}
where $N$ is the number of area elements in the discretized entangling surface
and $q$ is the flux through each area element. Putting everything together, the
edge mode partition function is found to be
\begin{equation}
  % \label{edge}
  Z_{\rm edge} = \int \prod_{\ell > 0, m} \frac{1}{q} \frac{1}{\sqrt{N}} dE_{\ell,
    m} \exp{-\sum_{\ell, m} \frac{\beta E_{\ell, m}^2}{2 \ell(\ell + 1) \sigma_0}}
  = \prod_{\ell > 0, m}\sqrt{\frac{2 \ell(\ell + 1) \sigma_0}{\beta N}}
  \frac{1}{q}.
\end{equation}
The associated entanglement entropy is
\begin{equation}
  \label{eq:edge-modes}
  S_{\rm edge} =\left. (1 - \beta \partial_{\beta}) \ln Z_{\rm edge} \right|_{\beta =
    2\pi} \sim \ln Z_{\rm edge}.
\end{equation}



\subsection{DW edge modes vs. conformally soft modes}
\label{sec:conf-soft-DW}

In this section we show that the edge modes of \cite{Donnelly:2014fua,
  Donnelly:2015hxa} are gauge equivalent to the logarithmic modes \cref{eq:log}
that are the building blocks of the conformally soft wavefunctions
\cref{eq:CS}.

% We start by comparing the conformally soft (or logarithmic) solutions of
% \cite{} with the edge modes of \cite{}.
We start by recalling that the Goldstone wavefunctions are defined by
\begin{equation}
  \label{eq:Goldstone-wf}
  A^{G}_{\mu;a} \equiv  \partial_{\mu} \alpha_a
\end{equation}
where $\alpha_a^{\pm}$ was defined in \cref{eq:cpw}. Meanwhile the logarithmic
wavefunctions take the form
\begin{equation}
  A^{\rm log \pm}_{\mu;a} = \log(-X^2 \mp i\varepsilon X^0) A^{G}_{\mu;a} .
\end{equation}
In the Milne coordinates \cref{eq:future-Milne}
\begin{equation}
  \log(-X^2) = \log(t^2 - r^2) = 2\tau
\end{equation}
and so in the future Milne wedge $-X^2 > 0$
\begin{equation}
  A^{\rm log }_{a} = 2 \tau d \alpha_a^{} =  2  \left(d(\tau \alpha_a^{}) - d\tau \alpha_a^{}\right).
\end{equation}
We hence see that the log solutions are gauge equivalent to the static Milne
solutions
\begin{equation}
  A_{\tau; a}^{} =  2 \alpha_a, ~~ A_{\sigma} = A_{w} = 0.
\end{equation}

We can explicitly check that near $\mathcal{I}^+$ the asymptotic expansions of
the static Milne solutions agree with the expansion of $\alpha_a.$ To this end,
it is convenient to introduce Poincar\'e coordinates
\begin{equation}
  e^{\sigma} = y.
\end{equation}
On the one hand, asymptotically as $y \rightarrow 0$, the static Milne solution
obeys the wave equation on $H_3$
\begin{equation}
  \label{eq:Poincare}
  y\partial_{y} \left(y^{-1} \partial_{y} A_{\tau}(y, w, \bw) \right) + 2 \partial_w\partial_{\bw} A_{\tau}(y,w,\bw) = 0.
\end{equation}
Moreover, near the boundary at $y = 0$, $A_{\tau}$ admits the expansion
\begin{align}
  A_{\tau}(y,w, \bw)
  &= \sum_{n = 0}^{\infty} \varphi_{2n}(w,\bw) y^{2n} + \sum_{n = 1}^{\infty} \varphi^{\rm log}_{2n}(w,\bw) y^{2n} \log y
\end{align}
and upon substitution into \cref{eq:Poincare} we find at the leading orders the
following recursion relations
\begin{align}
    y^0:~~~ &\varphi^{\rm log}_2 + \frac{1}{2}\Box_{\perp} \varphi_0 = 0,
              \label{eq:rec-rel1} \\
  y^2: ~~~ &4\varphi_4 + 3\varphi_4^{\rm log} +  \frac{1}{2}\Box_{\perp} \varphi_2 = 0,
             \label{eq:rec-rel2}\\
  y^2 \log y: ~~~ &4 \varphi^{\rm log}_4 + \frac{1}{2}\Box_{\perp} \varphi_2^{\rm log} = 0.
                    \label{eq:rec-rel3}
\end{align}
Here $\Box_{\perp} \varphi \equiv 2 \partial_w \partial_{\bw} \varphi.$ It is
straightforward to check that the first recursion relation is obeyed by
\cref{eq:ansatz,eq:radial}.



On the other hand, suppressing the dependence on the regulator $\pm i\reg$,
at large $r$ and fixed $u$ the gauge parameter $\alpha_z$ characterizing the
Goldstone wave functions becomes
\begin{equation}
  \label{eq:DPS}
  \frac{\varepsilon^+(z)\cdot X(w)}{q(z)\cdot X(w)} = \frac{(\bz-\bw ) r}{ r |w - z|^2 + u} = \frac{(\bz -\bw)y^{-1}}{|w - z|^2 y^{-1} + y}.
\end{equation}
Here we used
\begin{equation}
  r = e^{\tau - \sigma} = e^{\tau} y^{-1}, \quad
  u = e^{\tau + \sigma} = e^{\tau} y.
\end{equation}
As we expand \cref{eq:DPS} in the small $y \rightarrow 0$ limit we find
\begin{equation}
  \label{eq:soft-exp}
  \begin{split}
    \frac{\varepsilon^+(z)\cdot X(w)}{q(z)\cdot X(w)} &= \frac{1}{z - w} - \frac{y^2}{(\bz- \bw) (w - z)^2} + \mathcal{O}(y^4)\\
                                                      &-2\pi y^2 \log y \partial_z \left[\delta^{(2)}(z - w) + \cdots \right].
  \end{split}
\end{equation}
% Note that it was important to only keep the $e^{\rho}$ term as $r\rightarrow
% \infty$. Adding the $e^{-\rho}$ correction to $r$ leads to an expansion that
% doesn't obey \cref{eq:rec-rel1,eq:rec-rel2,eq:rec-rel3}. This is consistent
% with the approximation in \cref{eq:Poincare} which amounts to working in the
% Poincare patch.
For the contact terms we used the formula
% \begin{equation}
%\lim_{\phi \rightarrow \infty} \frac{1}{\pi} \frac{e^{-\phi}}{|z - w|^2 + e^{-2\phi}} = 2 \phi e^{-\phi} \delta^{(2)}(z - w) + \cdots 
%\end{equation}
\begin{equation}
  \begin{split}
    \frac{y}{y^2 + |z - w|^2} &\rightarrow \lim_{\phi \rightarrow \infty} \left[ \frac{e^{-\phi}}{e^{-2\phi} + |z - w|^2} + \frac{e^{-2\phi}}{(\bz - \bw)} \partial_{z} \left(\frac{e^{-\phi}}{e^{-2\phi} + |z - w|^2} \right) + \cdots \right] + \cdots \\
                              &= 2\pi \phi e^{-\phi} \delta^{(2)}(z - w) + 2\pi \phi e^{-3\phi} \frac{1}{\bz-\bw} \partial_{z} \delta^{(2)}(z - w) + \cdots .
  \end{split}
\end{equation}
We again see that \cref{eq:rec-rel1} is obeyed by the
expansion \cref{eq:soft-exp} as expected. Note that it was essential to include
the contact terms as well as the logarithmic terms in $y$, in the absence of
which the asymptotic expansion of \cref{eq:DPS} fails to satisfy the equations of
motion. The logarithmic terms in these expansions translate into logarithmic
terms in a large $r$ expansion of the gauge parameter in the Goldstone
wavefunction \cref{eq:Goldstone-wf} near $\mathcal{I}^+$ {\color{red} [But there
  seem to be no log terms in $A^{G}_{\mu}$ itself?]}. It would be interesting to
understand if these terms are related to the recently discovered logarithmic
corrections to the soft theorems \cite{}.



\subsection{Soft mode density matrix}
Our identification in section \ref{sec:conf-soft-DW} of conformally soft
{\color{red} [logarithmic]} modes with static electric fields in the Milne
region suggests that entanglement entropy of edge modes in \cref{eq:edge-modes}
can be identified with the entanglement entropy of conformally soft modes at
$\mathcal{I}^+$. In this section we show this is indeed the case. We start by
computing the reduced density matrix of conformally soft modes by tracing over
sectors of definite right Milne soft charge. We then evaluate the von Neuman
entropy of the resulting reduced density matrix. The result remarkably agrees
with the edge mode entropy computed in \cite{Donnelly:2014fua, Donnelly:2015hxa}
with different methods.

The reduced density matrix of conformally soft modes is defined by
\begin{equation}
  \rho_L \equiv \int \mathcal{D}q_R \langle q_R| \rho| q_R\rangle 
\end{equation}
where $|q_R\rangle$ is a state of definite right Milne charge
\begin{equation}
  \label{eq:fixed-right-charge-state}
  \hat{Q}^R_a |q_R \rangle = q^R_a |q_R\rangle
\end{equation}
% and $\hat{\mathscr{S}}_L$ is the Goldstone operator for the left Milne patch.
The right Milne charges are defined in analogy with the soft charge at
$\mathcal{I}^+$ by
\begin{equation}
  \hat{Q}^R_a \equiv-i \langle \widetilde{A}^{\confDim = 1, R}_{a;\mu},A^{\mu} \rangle.
\end{equation}
Note that the net soft charge is
\begin{equation}
  \label{eq:net-soft}
  \hat{Q}_a \equiv  -i\langle \widetilde{A}^{\confDim = 1}_{a;\mu}, A^{\mu} \rangle = \hat{Q}^L_a + \hat{Q}^R_a,
\end{equation}
which follows from the fact that $A^L$ and $\widetilde{A}^R$ vanish in the right
and left Milne patches respectively. {\color{red}[Comment on the net large gauge
  charge]} As we will show below, the projection $\langle q_R| \rho| q_R\rangle$
onto a state of fixed net large Milne charge renders $\rho_L$ a functional of
the Goldstone operator
\begin{equation}
  \hat{\mathscr{S}}^L_a \equiv  -i \langle A^{\mu}, \widetilde{A}_{a;\mu}^{CS, L}\rangle.
\end{equation}
The AdS/CFT dictionary on the AdS$_3$ Milne slices allows us to identify the
conformally soft mode partition function with the path integral over Goldstone
modes $\hat{\mathscr{S}^L}$ on the celestial sphere
\begin{equation}
  \left. Z_{CS}\right|_{\beta = 2\pi} = \int \mathcal{D}\mathscr{S} \rho_L[\mathscr{S}].
\end{equation}
The entanglement entropy of conformally soft modes is then given by {\color{red}
  [restore $\beta$ to be able to define this...?]}
\begin{equation}
  % \label{eq:Scs1}
  S_{CS} \equiv .
\end{equation}


As a first step in evaluating the entanglement entropy of conformally soft modes
\cref{eq:Scs2}, we need to construct a state of definite right Milne
charge satisfying \cref{eq:fixed-right-charge-state}. Following \cite{}, such states are
obtained by adapting the construction of Dirac/Chung/Kibble/Faddeev-Kulish
dressed states \cite{Dirac:1955uv,Chung:1965zza, Kibble:1968lka, Kibble:1968npb,
  Kibble:1968oug, Kulish:1970ut, Kapec:2017tkm, Arkani-Hamed:2020gyp} namely
\begin{equation}
  \label{eq:right-charge}
  |q_R\rangle = \exp\left\{\int d^2 z \sqrt{{\rm det}\celMet} q_R^a(z, \bz) \hat{\mathscr{S}}_{a}^R(z,\bz)\right\} |0\rangle_R.
\end{equation}
Here
\begin{equation}
  \hat{\mathscr{S}}_{a}^R \equiv-i \langle \widetilde{A}_{a;\mu}^{CS, R},  A^{\mu}\rangle
\end{equation}
is the right Milne Goldstone operator canonically conjugate to
$\hat{\mathscr{Q}}^R_a$
\begin{equation} [\hat{\mathscr{Q}}^R_a, \hat{\mathscr{S}}^R_b] = 2\pi i\int d^2
  w \partial_a \partial_b \log|z - w|^2
\end{equation}
{\color{red} Fix prefactor.}
It follows immediately from the property \eqref{} of coherent states together
with
\begin{equation}
  \hat{\mathscr{Q}}_a^R|0\rangle_R = 0
\end{equation}
that the state \cref{eq:right-charge} diagonalizes the right Milne soft charge
as in \cref{eq:fixed-right-charge-state}. In particular, we find
\begin{equation}
  \hat{Q}_b^{R}(z)|q_R\rangle = 2\pi i \int d^2 w \sqrt{{\rm det}\celMet} q^a_R(w,\bar{w}) \partial_a\partial_{b} \log|z - w|^2.
\end{equation}

Moreover, using \eqref{} in appendix \ref{} we find that
\begin{equation}
  \langle q_R| \rho |q_R \rangle = |\Psi_L\rangle \langle \Psi_L| 
\end{equation}
where
\begin{equation}
  |\Psi_L\rangle = N \exp\left\{\int_0^{\infty} d\milneFreq \int d^2z \sqrt{{\rm det}\celMet} e^{-\pi \milneFreq} (\celMet)^{c\bar{d}}a_{c, \milneFreq}^{L\dagger} \int d^2 z' \sqrt{{\rm det}\celMet'} q_R^{a*}(z', \bz') [\hat{\mathscr{S}}_{a}^{R\dagger}(z',\bz'), \widetilde{a}^{R\dagger}_{d,\milneFreq}(z,\bz)]\right\}| 0 \rangle_L .
\end{equation}

On the one hand, in \cref{app:left-right-Milne} we find that
\begin{equation}
  \begin{split}
    \lim_{\confDim \rightarrow 1} \partial_{\confDim}\left[\langle A^{+L \confDim}_{a;\mu}(q), A_{\mu}\rangle - \langle A^{-L \confDim}_{a;\mu}(q), A_{\mu}\rangle\right] &= - \frac{i e}{2}\int_0^{\infty} \diff\celFreq \left[ a_a(\celFreq \nullUnit) - a_a^{\dagger}(\celFreq\nullUnit) \right],\\
    \lim_{\confDim \rightarrow 1} \partial_{\confDim}\left[\langle A^{+R \confDim}_{a;\mu}(q), A_{\mu}\rangle - \langle A^{-R \confDim}_{a;\mu}(q), A_{\mu}\rangle \right] &= -  \frac{i e}{2}\int_0^{\infty} \diff\celFreq \left[a_a(\celFreq \nullUnit) - a_a^{\dagger}(\celFreq\nullUnit) \right].
  \end{split}
\end{equation}
We hence find the mode expansion of the Goldstone operator in terms of plane
wave modes
\begin{equation}
  \hat{\mathscr{S}}_a^R =  \frac{ie}{4\pi}\int_0^{\infty} \diff\celFreq \int \frac{d^2 w}{2\pi} \sqrt{{\rm det}\celMet}  \partial_a\p^b \log|z - w|^2 \left[a_{b}(\celFreq , w) - a^{\dagger}_{\bar{b}}(\celFreq, w) \right].
\end{equation}
On the other hand, using the Bogoliubov relations \cref{eq:Bogo} together with
the expansion \cref{eq:pw-cpw} of plane wave modes in terms of conformal primary
ones, we find the commutators
\begin{equation}
  \begin{split}
    [\widetilde{a}_{a,\milneFreq}^{R\dagger}(q), a_b(\celFreq q')] &\propto (\celMet)_{a\bar{b}} \frac{\sqrt{1 + \milneFreq^2}}{4\pi \sqrt{\milneFreq} \sinh\pi \milneFreq}\frac{1}{(1 - i\milneFreq) \Gamma(-i\milneFreq)}  \celFreq^{-i\milneFreq - 1} 2 (2\pi)^3 \delta^{(2)}(z - z'), \\
    [\widetilde{a}_{a,\milneFreq}^{R\dagger}(q), a_b^{\dagger}(\celFreq q')] &\propto (\celMet)_{a\bar{b}} \frac{\sqrt{1 + \milneFreq^2}}{4\pi \sqrt{\milneFreq} \sinh\pi \milneFreq}\frac{1}{(1 + i\milneFreq) \Gamma(i\milneFreq)}  \celFreq^{i\milneFreq - 1} 2 (2\pi)^3 \delta^{(2)}(z - z').
  \end{split}
\end{equation}
{\color{red} Figure out proportionality constant after making sure all normalization constants are correct.}
We hence conclude that
\begin{equation}
  \label{eq:cpw-Goldstone}
  [\widetilde{a}_{a, \milneFreq}^{R\dagger}(z), \hat{\mathscr{S}}^R_b(z')] \propto  -\frac{1}{\sqrt{\milneFreq}} \delta(\milneFreq) 2\pi \partial_a\partial_{\bar{b}} \log|z - z'|^2.
\end{equation}

Putting everything together, $|\Psi_L\rangle$ reduces to
\begin{equation}
  \label{eq:Left}
  |\Psi_L\rangle = N \exp\left\{\lim_{\epsilon \rightarrow 0} \frac{1}{\sqrt{\epsilon}}\int d^2z \sqrt{{\rm det}(\celMet)_z} \int d^2 w \sqrt{{\rm det}(\celMet)_w} 2\pi \partial_a\partial_{\bar{b}}\log|z - w|^2 q_R^{a*}(z,\bz) a_{L,\milneFreq = \epsilon}^{\bar{b}\dagger}(w,\bw)\right\}|0\rangle_L.
\end{equation}
Since
\begin{equation}
  q_R^a + q_L^a = \cdots
\end{equation}
and using the identification of $q_L^a$ with the static solutions in the Milne
patch established in section \ref{} we see that the von Neuman entropy of
the state \cref{eq:Left} ought to coincide with the entanglement entropy of edge modes
\eqref{} {\color{red}[need to finish this]}. The large $\rho$ cutoff $\rho_0$ in
\eqref{} manifests here as the infrared regulator $\epsilon$ arising from the
pole at $\milneFreq = 0$ in \cref{eq:cpw-Goldstone}.


Equivalently, the classical probability distribution associated with a state of
definite right (and by \cref{eq:net-soft}, for fixed net soft charge, left) Milne
charge is
\begin{equation}
  p(q_R) \equiv \int \mathcal{D}\mathscr{S} \langle q_R| \rho| q_R\rangle.
\end{equation}
The conformally soft mode entanglement entropy is then given by
\begin{equation}
  \label{eq:Scs2}
  S_{CS} \equiv -\int \mathcal{D} q_R p(q_R) \log p(q_R).
\end{equation}
This formula is the analog of \cref{eq:edge-modes} since
\begin{equation}
\end{equation}
{\color{red} [use AdS-CFT dictionary on the hyperbolic Milne slices to argue these two are equivalent.]}


\subsection{Celestial CFT and Goldstone vertex operators}



%%% Local Variables:
%%% mode: latex
%%% TeX-master: "../main"
%%% End:
